# Supplementary material for: Self-Supervised Multi-Object Tracking For Autonomous Driving From Consistency Across Timescales
Source: arXiv:2304.13147 source file (2023-09-21)
Supplement: Supplementary file 1 [file 62_supp_degenerate_cases.tex]

\subsection{Discussion degenerate cases}

The self-supervised learning task proposed in the main paper can be ill-defined for specific configurations.
One such scenario is given when no two object detections in a sequence correspond to each other. In this configuration, all tracks are deleted, which leaves no associations to compute a loss value for.
Such a scenario is possible, e.g. with large camera rotation between frames, such that the  field of views of the initial and final camera perspectives have zero overlaps. For the datasets used in our paper, \ie \gls{mot17} and \gls{bdd}, we, therefore, performed an overlap analysis of the annotated subsets, which is depicted in \figref{}.
For this analysis, we computed the histogram of track lengths for the entire dataset and each split separately on the left side. 
The right side shows the union ratios of track IDs between all frames for variable sequence lengths.
We find that the dataset does not contain the potential for such degenerate cases.
Therefore, such degenerate cases would only arise when the object detector outputs imperfect predictions. In such cases, we skip parameter updates for this sample.

\begin{table*}[]
\scriptsize
\centering
\caption{Dataset track statistics for the \gls{bdd} and \gls{mot17} annotations. Overlap is computed for a sequence length of $N=4$ and $N=8$ respectively.}
\label{tab:dataset_stats}
\begin{tabular}{c|cccc|cccc|cccc|cccc} \toprule
 & \multicolumn{4}{c|}{instances per frame} & \multicolumn{4}{c|}{Overlap (N=4) [\%]} & \multicolumn{4}{c|}{Overlap (N=8)[\%]} & \multicolumn{4}{c}{Track length} \\ 
 & q=5\% & q=95\% & mean & std & q=5\% & q=95\% & mean & std & q=5\% & q=95\% & mean & std & q=5\% & q=95\% & mean & std \\ \midrule
BDD100k train & 2 & 57 & 9.98 & 5.84 & 44.4 & 100.0 & 77.7 & 18.6 & 25.0 & 100.0 & 65.7 & 22.4 & 2 & 203 & 18.54 & 26.21 \\
BDD100k val & 2 & 49 & 11.25 & 6.85 & 45.5 & 100.0 & 77.1 & 18.2 & 27.3 & 100.0 & 65.1 & 21.6 & 1 & 203 & 17.94 & 25.80 \\ \midrule
MOT17 half-train & 7 & 49 & 21.92 & 13.44 & 81.8 & 100.0 & 96.2 & 6.5 & 72.7 & 100.0 & 93.2 & 9.1 & 7 & 526 & 162.69 & 157.92 \\
MOT17 train & 6 & 52 & 21.12 & 14.34 & 81.8 & 100.0 & 95.9 & 7.2 & 71.4 & 100.0 & 92.6 & 10.1 & 7 & 1050 & 205.29 & 256.19 \\
MOT17 half-val & 5 & 52 & 20.32 & 15.15 & 81.8 & 100.0 & 95.6 & 7.9 & 69.8 & 100.0 & 92.0 & 11.0 & 8 & 524 & 158.49 & 157.13 \\ \bottomrule
\end{tabular}
\end{table*}

We would like to point out, that most self-supervised pre-training task suffers from some sort of edge cases, that results in degenerate loss computation. 
For example, image augmentations like cropping used in almost all contrastive approaches could remove the principal object from the image, if it is located at a border region and not occupying sufficient areas of the image.

In our case, we could filter out such scenarios, where a pre-trained tracker loses all tracks within the length of a sample sequence. Another scenario would be to pre-train our method on examples, where we can ensure that all tracks survive the sample length. Then, this self-supervised tracker is trained on a curated subset of the training data to perform the filtering.
