# Supplementary material for: Self-Supervised Multi-Object Tracking For Autonomous Driving From Consistency Across Timescales
Source: arXiv:2304.13147 source file (2023-09-21)
Supplement: Supplementary file 2 [file 61_supp_assigner.tex]

\begin{table*}[]
\scriptsize
\centering
\caption{Assignment error of various approximate bipartite matching methods compared to optimal cost assignment by Hungarian algorithm~\cite{hungarianmethod}. Results are calculated for 1000 runs on random cost matrices sampled from the interval $[0, 1]$, and runtimes are reported as average. $h$ represents the threshold for assigning to the insertion/deletion class.}
\label{tab:supp_matcher_testbed}
\begin{tabular}{cccccccccc} \toprule
Method & $[0, 1]^{n \times m }$& \multicolumn{2}{c}{h = 0.0} & \multicolumn{2}{c}{h = 0.25} & \multicolumn{2}{c}{h = 0.5} & \cite{brun2022lsape} [ms] & HM~\cite{hungarianmethod}[ms] \\ 
 & & $\mu$ & $\sigma^2$ & $\mu$ & $\sigma^2$ & $\mu$ & $\sigma^2$  &  &  \\ \midrule
\multirow{4}{*}{\cite{brun2022lsape}} & 10 $\times$ 10 & 33.11 & 43.08 & 21.59 & 46.32 & 11.68 & 26.19 & 0.70 & 0.08 \\
 & 10 $\times$ 20 & 46.12 & 63.72 & 27.02 & 65.41 & 25.26 & 65.89 & 0.41 & 0.08 \\
 & 20 $\times$ 20 & 34.32 & 21.60 & 33.12 & 23.34 & 14.00 & 24.77 & 1.08 & 0.15 \\
 & 20 $\times$ 30 & 45.09 & 28.44 & 35.20 & 28.35 & 35.52 & 31.32 & 0.61 & 0.14 \\ \midrule
\multirow{4}{*}{BPMN} & 10 $\times$ 10 & 11.13 & 13.25 & 10.09 & 13.01 & 9.32 & 12.94 & 0.34 & 0.08 \\
 & 10 $\times$ 20 & 10.92 & 13.03 & 10.81 & 12.73 & 11.78 & 12.18 & 0.34 & 0.08 \\
 & 20 $\times$ 20 & 11.35 & 10.12 & 11.08 & 9.78 & 11.43 & 10.09 & 0.37 & 0.15 \\
 & 20 $\times$ 30 & 8.81 & 10.13 & 8.18 & 10.75 & 7.30 & 10.67 & 0.58 & 0.14 \\
 \bottomrule
\end{tabular}
\end{table*}
