# Supplementary material for: Self-Supervised Multi-Object Tracking For Autonomous Driving From Consistency Across Timescales
Source: arXiv:2304.13147 source file (2023-09-21)
Supplement: Supplementary file 3 [file supp_dataset_track_stats.tex]

\begin{table*}[]
\scriptsize
\centering
\caption{Dataset track statistics for the \gls{bdd} and \gls{mot17} annotations. Overlap is computed for a sequence length of $N=4$ and $N=8$ respectively.}
\label{tab:dataset_stats}
\begin{tabular}{c|cccc|cccc|cccc|cccc} \toprule
 & \multicolumn{4}{c|}{instances per frame} & \multicolumn{4}{c|}{Overlap (N=4) [\%]} & \multicolumn{4}{c|}{Overlap (N=8)[\%]} & \multicolumn{4}{c}{Track length} \\ 
 & q=5\% & q=95\% & mean & std & q=5\% & q=95\% & mean & std & q=5\% & q=95\% & mean & std & q=5\% & q=95\% & mean & std \\ \midrule
BDD100k train & 2 & 57 & 9.98 & 5.84 & 44.4 & 100.0 & 77.7 & 18.6 & 25.0 & 100.0 & 65.7 & 22.4 & 2 & 203 & 18.54 & 26.21 \\
BDD100k val & 2 & 49 & 11.25 & 6.85 & 45.5 & 100.0 & 77.1 & 18.2 & 27.3 & 100.0 & 65.1 & 21.6 & 1 & 203 & 17.94 & 25.80 \\ \midrule
MOT17 half-train & 7 & 49 & 21.92 & 13.44 & 81.8 & 100.0 & 96.2 & 6.5 & 72.7 & 100.0 & 93.2 & 9.1 & 7 & 526 & 162.69 & 157.92 \\
MOT17 train & 6 & 52 & 21.12 & 14.34 & 81.8 & 100.0 & 95.9 & 7.2 & 71.4 & 100.0 & 92.6 & 10.1 & 7 & 1050 & 205.29 & 256.19 \\
MOT17 half-val & 5 & 52 & 20.32 & 15.15 & 81.8 & 100.0 & 95.6 & 7.9 & 69.8 & 100.0 & 92.0 & 11.0 & 8 & 524 & 158.49 & 157.13 \\ \bottomrule
\end{tabular}
\end{table*}
